# Supplementary material for: Rate-Splitting Random Access Mechanism for Massive Machine Type Communications in 5G Cellular Internet-of-Things
Source: arXiv:2106.14621 source file (2021-06-08)

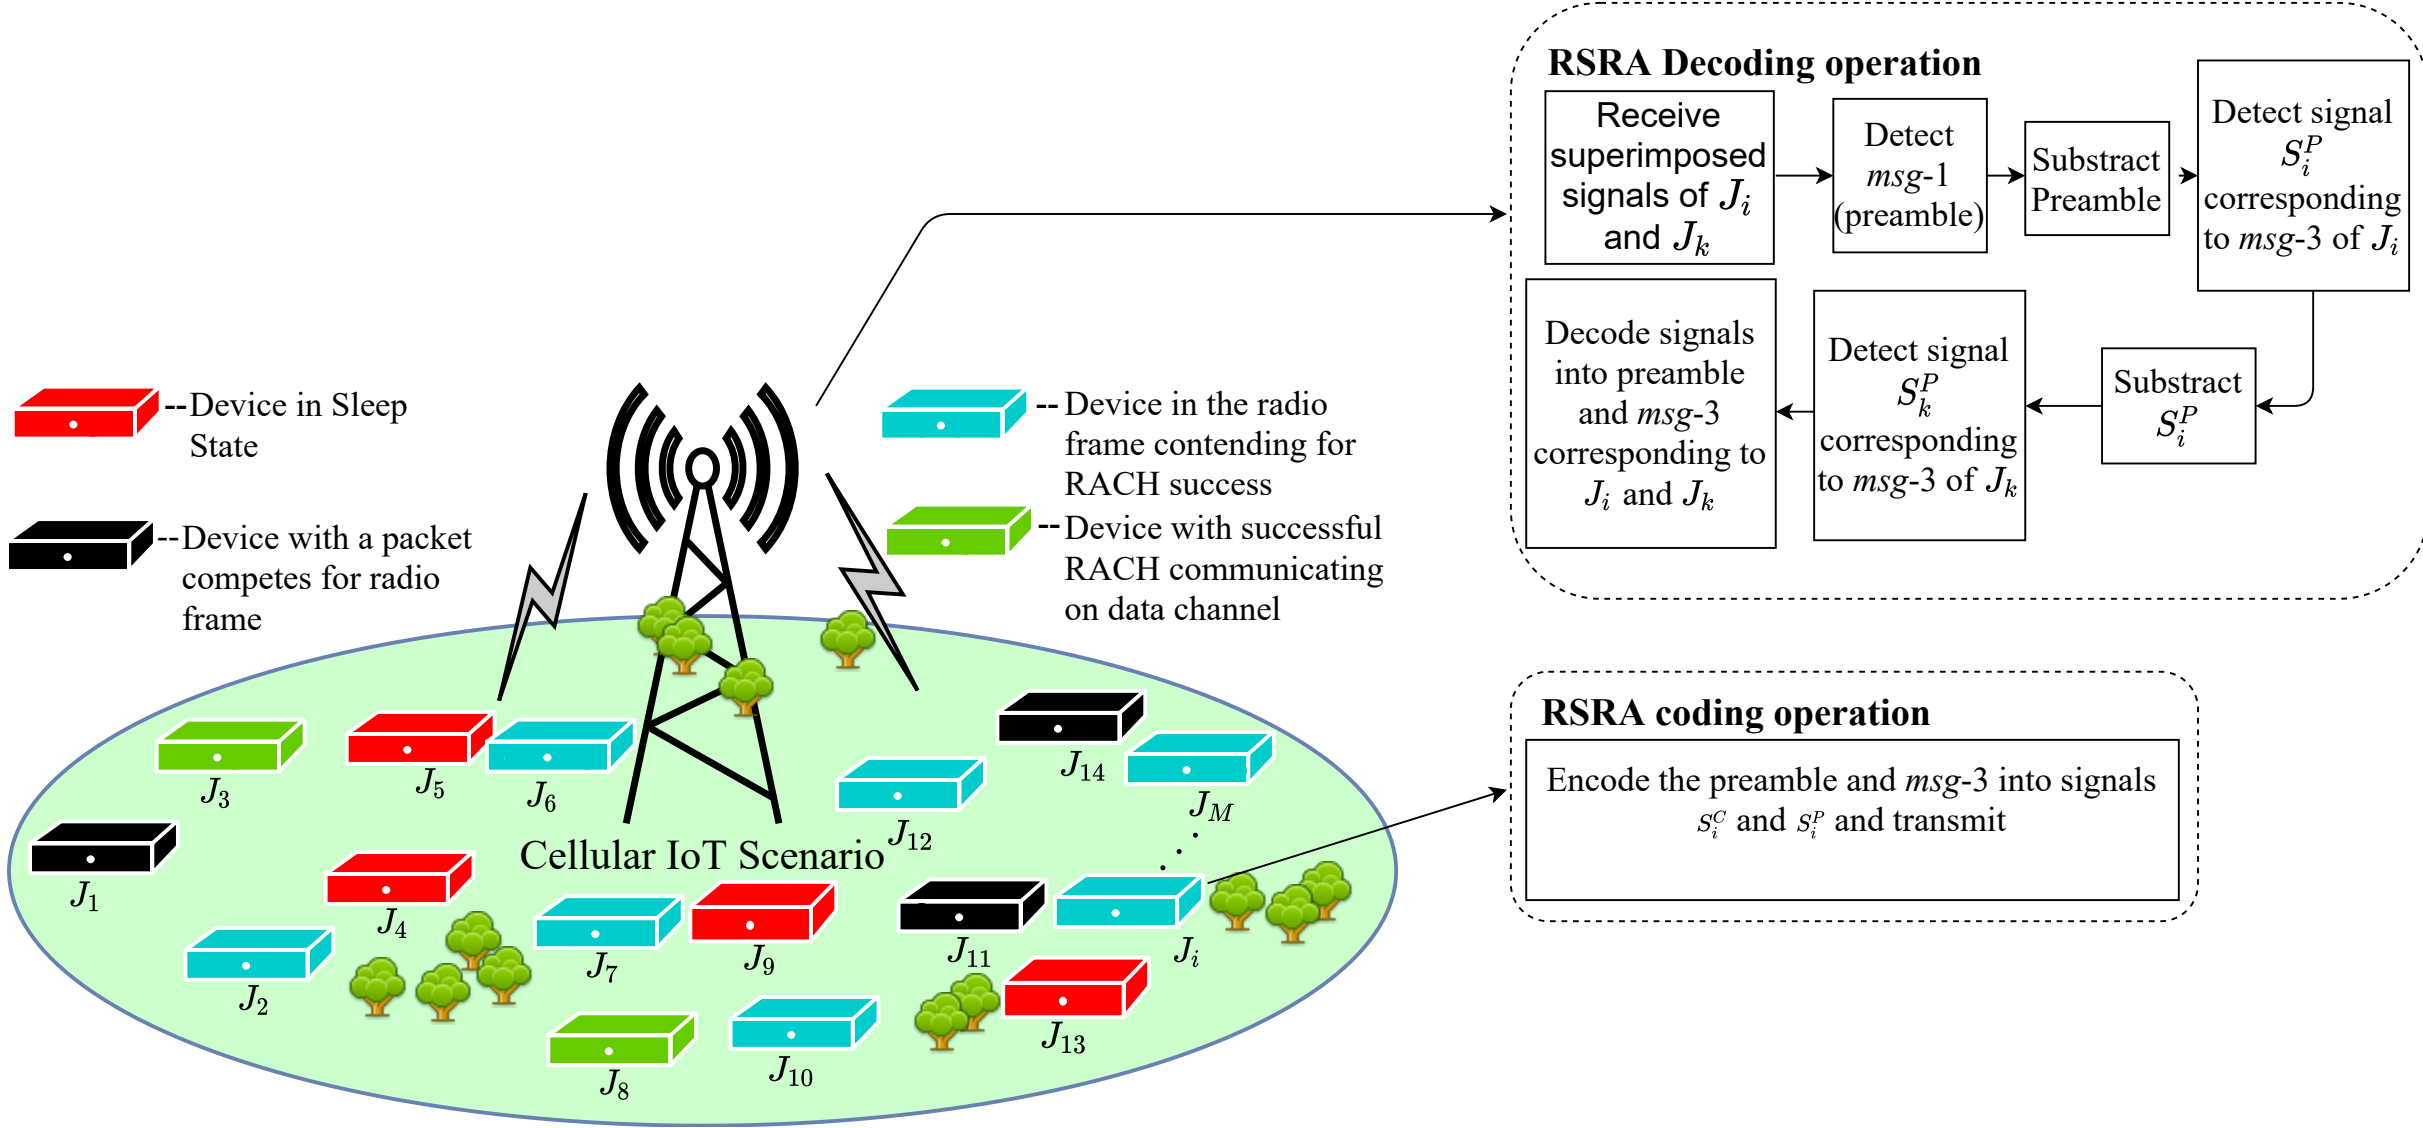

Supplement: Supplementary file 1 [file sm_RSMA.pdf]
